# Supplementary material for: Nonlinear Temperature Sensitivity of Residential Electricity Demand: Evidence from a Distributional Regression Approach
Source: arXiv:2503.07213 source file (2025-03-10)
Supplement: Supplementary file 1 [file 06_FRKET_APPENDIX.tex]

\section{Asymptotic analysis}\label{sec_app_est}
\subsection{Preliminaries} \label{sec_app_prelim}
We let $\mathcal H_1$ a separable Hilbert space with inner product $\langle \cdot,\cdot \rangle_1$ %(e.g., the $L^2[0,1]$ space of square integrable functions) 
and norm $\|\cdot\|_1$. A $\mathcal H_1$-valued random variable $Z$ is defined as a measurable map from the underlying probability space to $\mathcal H_1$. Such a random element $Z$ is said to be square-integrable if $\mathbb{E}[\|Z\|_1^2<\infty]$. Let $\mathcal H_2$ be another such Hilbert space. We let $\otimes$ denotes the tensor product defined by $\mathcal H_1$ and $\mathcal H_2$, i.e., for any $\zeta_1 \in \mathcal H_1$ and $\zeta_2 \in \mathcal H_2$, 
\begin{equation}
\zeta_1\otimes \zeta_2 (\cdot) = \langle \zeta_1,\cdot \rangle \zeta_2; 
\end{equation}
note that $\zeta_1\otimes \zeta_2$ is a map from $\mathcal H_1$ to $\mathcal H_2$. 

For any mean-zero square-integrable random elements $Z_1$ and $Z_2$, $\mathbb{E}[Z_1 \otimes Z_2]$ is called the covariance operator of $Z_1$ and $Z_2$. We call $A:\mathcal H_1 \mapsto \mathcal H_2$ a bounded linear map if $A$ is a linear map and its operator norm, defined as $\|A\|_{\op}=\sup_{|\zeta|\leq 1} \|A\zeta\|$, is finite. For any bounded linear $A$, we let $A^\ast$ be the adjoint map defined by the property $\langle A\zeta_1,\zeta_2 \rangle_2=\langle \zeta_1,A^\ast\zeta_2 \rangle_1$ for all $\zeta_1\in \mathcal H_1$ and $\zeta_2 \in \mathcal H_2$.  We say that $A$ is a compact operator if $\mathcal H_1=\mathcal H_2$ and there exist orthonormal bases $\{\zeta_{1,j}\}_{j\geq 1}$ and $\{\zeta_{2,j}\}_{j\geq 1}$ such that $A = \sum_{j=1}^\infty a_j \zeta_{1,j} \otimes \zeta_{2,j}$ with $a_j$ tending to zero as $j$ increases; in this expression, if $A$ is self-adjoint ($A=A^\ast$) and nonnegative ($\langle A\zeta,\zeta \rangle_1\geq 0$), it may be assumed that $a_j\geq 0$ and $\zeta_{1,j}=\zeta_{2,j}$, and furthermore they are understood as the eigenvalues and the corresponding eigenvectors. A compact operator $A$ is Hilbert-Schmidt if $\sum_{j=1}^\infty \|A \zeta_j\|_1^2 < \infty$ for some orthonormal basis $\{\zeta_j\}_{j\geq1}$, and in this case, the Hilbert-Schmidt norm $\|A\|_{\HS}$ is defined as  $\|A\|_{\HS}= \sqrt{\sum_{j=1}^\infty \|A \zeta_j\|_1^2}$. It is well known that $\|A\|_{\op} \leq \|A\|_{\HS}$.

\subsection{Functional IV estimator in the FSR model} \label{sec_app_est_1}
We consider a suitable adaptation of the functional IV estimator (FIVE) proposed by \cite{seong2021functional} for our FSR model.
 We find that for an IV $Z_t$ satisfying \eqref{eqreg3}, we find from \eqref{eqreg2} that $C_{Zy} = fC_{XZ}^\ast$ and hence 
\begin{align} \label{eqpopulation}
 C_{Zy}C_{XZ} = f C_{XZ}^\ast C_{XZ},
\end{align}
where $C_{Zu}:=\mathbb{E}[(Z_t-\mathbb{E}[Z_t])\otimes u_t]=0$.
As in \cite{seong2021functional} studying on the FFR model, we construct an estimator mimicking the population relationship \eqref{eqpopulation}. We first replace $C_{Zy}C_{XZ}$ and $C_{XZ}^\ast C_{XZ}$ given in \eqref{eqpopulation} with their sample counterparts $\widehat C_{Zy}\widehat C_{XZ}$ (where $\widehat C_{Zy}=T^{-1}\sum_{t=1}^T (Z_t-\bar{Z}_T)\otimes (y_t-\bar{y}_T)$ with $\bar{y}_T=T^{-1}\sum_{t=1}^T y_t$) and $\widehat  C_{XZ}^\ast \widehat C_{XZ}$. We then employ a regularized inverse of $\widehat  C_{XZ}^\ast \widehat C_{XZ}$ to compute an estimator from the sample equation. Specifically, as in \cite{seong2021functional}, we consider the rank-regularized inverse $(\widehat{C}_{XZ}^\ast \widehat{C}_{XZ})^\dag$ of $\widehat{C}_{XZ}^\ast \widehat{C}_{XZ}$ is defined as follows:
\begin{equation} \label{eqregul}
(\widehat{C}_{XZ}^\ast \widehat{C}_{XZ})^\dag =  \sum_{j=1}^{\KK} {\hat{\lambda}_j^{-2}} \hat{g}_j \otimes \hat{g}_j,
\end{equation}
where $\KK$ is determined as 
\begin{equation} \label{eqchoicek}
\KK = \max_{j\geq 1} \{\hat{\lambda}_j^2 \geq \alpha\}
\end{equation}
for some $\alpha$ tending to zero. Note that $\widehat{C}_{XZ}^\ast \widehat{C}_{XZ}(\widehat{C}_{XZ}^\ast \widehat{C}_{XZ})^\dag$  becomes the $\KK$-dimensional projection $\widehat{\Pi}_{\KK} = \sum_{j=1}^{\KK} \hat{g}_j \otimes \hat{g}_j$ and similar regularized inverses are widely used in the literature on the functional linear model. The estimator $\hat{f}$ is defined as follows: for any $x \in \mathcal H$
\begin{align} \label{eqest1}
\hat{f} (x)=  \widehat{C}_{Zy} \widehat{C}_{XZ} (\widehat{C}_{XZ}^\ast \widehat{C}_{XZ})^\dag (x).
\end{align}
With some algebra, it can be shown that \eqref{eqest1} is identical to the expression given by \eqref{eqest}.   
\begin{remark} \label{rem1}
The choice $\KK$ in \eqref{eqchoicek} is adopted from \cite{seong2021functional} concerning the FFR model. Of course, with only a minor modification, we can obtain the desired asymptotic results— which will be discussed—under an alternative choice, such as $\KK = m +  \max_{j\geq 1}\{\hat{\lambda}_j^2 \geq \alpha\}$ for some finite $m$, if necessary. This choice may be preferred when researchers want to retain at least $m$ eigenelements for estimation. The case with $m=1$ also has some theoretical justification, given that we need at least one eigenelement for the proposed estimator to be well defined for every $T$.
\end{remark}
\subsection{Consistency and local asymptotic normality of the estimator}\label{sec_app_est_2}
This section discusses the consistency and local asymptotic normality of the proposed estimator, which are fundamental for our empirical analysis. As in \cite{seong2021functional}, for simplicity, we consider the case where $y_t$, $X_t$, and $Z_t$ have zero means, so the regression model \eqref{eqreg1} simplifies to $y_t = f(X_t^{\circ}) + \varepsilon_t$. In this case, the population (e.g., $C_{XZ}$) or sample covariance operators (e.g., $\widehat{C}_{XZ}$)  introduced in Section \ref{sec_method} are naturally understood as defined without centering or demeaning. As discussed in \cite{seong2021functional}, extending the subsequent results to the case where the means are unknown and need to be estimated is straightforward, and the consistency and local asymptotic normality to be established remain unchanged with or without this simplification. 

\subsubsection{Assumptions and main results}
 Hereafter, we let
\begin{equation}
C_{XZ}^\ast C_{XZ} = \sum_{j=1}^\infty \lambda_j^2 g_j \otimes g_j, \quad C_{XZ} C_{XZ}^\ast = \sum_{j=1}^\infty \lambda_j^2 h_j \otimes h_j,
\end{equation}
where $\lambda_j$, $g_j$, and $h_j$ are relevant eigenelements. Let $C_{ZZ}=\mathbb{E}[Z_t\otimes Z_t]$, $C_{uu}=\mathbb{E}[u_t\otimes u_t]$ and $C_{Zu}=\mathbb{E}[Z_t\otimes u_t]$. We define $\widehat{C}_{ZZ}$, $\widehat{C}_{uu}$ and $\widehat{C}_{Zu}$ be defined as follows:
\begin{equation}
\widehat{C}_{ZZ}=T^{-1}\sum_{t=1}^T Z_t\otimes Z_t, \quad \widehat{C}_{uu}=T^{-1}\sum_{t=1}^T u_t\otimes u_t, \quad  \widehat{C}_{Zu}=T^{-1}\sum_{t=1}^T Z_t\otimes u_t,
\end{equation}
which may be understood as the sample counterparts of $C_{ZZ}$, $C_{uu}$ and $C_{Zu}$. We employ the following assumptions: below, $\mathfrak{F}_t$ denotes the natural filtration given by $\sigma(\{Z_s\}_{s\leq t+1}, \{u_s\}_{s\leq t})$ and let $\tau_j = 2\sqrt{2} \max\{ (\lambda_{j-1}^2-\lambda_j^2)^{-1}, (\lambda_{j}^2-\lambda_{j+1}^2)^{-1} \}$ as in \cite{seong2021functional}.
\begin{assumption}\label{assum1}
\begin{enumerate*}[(i)]
\item Equation \eqref{eqreg2} holds; \item $\{X_t,Z_t\}_{t\geq 1}$ is stationary and geometrically strongly mixing, $\mathbb{E}[\|X_t\|^2] < \infty$, and $\mathbb{E}[\|Z_t\|^2] < \infty$; \item $\mathbb{E}[u_t|\mathfrak F_{t-1}]=0$,  $\mathbb{E}[u_t \otimes u_t|\mathfrak F_{t-1}]=C_{uu}$, and $\sup_{1\leq t\leq T}\mathbb{E}[\|u\|_t^{2+\delta}|\mathfrak F_{t-1}] < \infty$ for some $\delta>0$; \item $\sum_{j=1}^\infty |f(b_j)|^2 < \infty$ for some orthonormal basis $\{b_j\}_{j\geq 1}$ of $\mathcal H$; \item $\|\widehat{C}_{XZ}-{C}_{XZ}\|_{\HS}=O_p(T^{-1/2})$, $\|\widehat{C}_{ZZ}-{C}_{ZZ}\|_{\HS}=O_p(T^{-1/2})$,  $\|\widehat{C}_{Zu}-{C}_{Zu}\|_{\HS}=O_p(T^{-1/2})$ and $\|\widehat{C}_{uu} - C_{uu}\|_{\HS}= o_p(1)$; \item $\ker C_{XZ}=\{0\}$; \item \label{eq001a1}$\lambda_1^2 > \lambda_2^2 > \cdots > 0$; \item $T^{-1}\alpha^{-1} \to 0$ and $T^{-1/2}\sum_{j=1}^{\KK} \tau_j \to_p 0$. 
\end{enumerate*}
\end{assumption}
The conditions given in Assumption \ref{assum1} are adapted from Assumptions M and E of \cite{seong2021functional} studying the FFR model, and similar assumptions have been employed in  the literature on functional linear models. Condition \ref{eq001a1} is a technical requirement that $\alpha$ decay at an appropriate rate depending on the eigenvalues $\{\lambda_j\}_{j\geq 1}$ and $T$. This subtle requirement on $\alpha$ may be relaxed if some additional (but standard in the literature on the functional linear model) assumptions are employed, which will be discussed later in this section. %it is common to assume that $\lambda_j^2 - \lambda_{j+1}^2$ is eventually convex and bounded above by $O(j^{\gamma})$ for some $\gamma > 3$ (see Assumption 2 below and also Assumption E2 of \citealp{seong2021functional}). In this case, $T^{-1/2}\sum_{j=1}^{\KK} \tau_j \leq  O_p(T^{-1/2}\KK4)$ the assumption  
 We then present the following consistency result, which details Proposition \ref{prop1} given in Section \ref{Sec_Model}:
\begin{proposition} \label{prop1a}
Under Assumptions \ref{assum1}, $\|\hat{f} - f\|_{\op} \to_p 0$.  
\end{proposition}

We next obtain the local asymptotic normality result \eqref{eqlocal} for any specified $\zeta \in \mathcal H$. To this end, we employ the following assumptions: below, we let $\upsilon_{t}(j,\ell) = \langle X_t,g_j \rangle\langle Z_t,h_{\ell}\rangle -\mathbb{E}[\langle X_t,g_j \rangle\langle Z_t,h_{\ell}\rangle]$ for $j,\ell \geq 1$ and $\theta_{\KK}(\zeta)= \langle \tilde{\zeta}, {C}_{ZZ} \tilde{\zeta}  \rangle$, where $\tilde{\zeta} = \sum_{j=1}^{\KK} {\lambda}_j^{-2} \langle {g}_j,\zeta \rangle {C}_{XZ}{g}_j$.

\begin{assumption}\label{assum2} For some $c_\circ>0$, $\rho>2$, $\varsigma>1/2$, $\delta_{\zeta}>1/2$ and $m>1$, the following holds:
\begin{enumerate*}[(i)]
\item $\lambda_j^2 \leq c_\circ j^{-\rho}$; \item $\lambda_j^2-\lambda_{j+1}^2 \geq c_\circ j^{-\rho-1}$; \item $|f(g_j)| \leq c_\circ j^{-\varsigma}$; \item $\mathbb{E}[\upsilon_t(j,\ell)\upsilon_{t-s}(j,\ell)] \leq c_\circ s^{-m}\mathbb{E}[\upsilon_t^2(j,\ell)]$ for $s\geq 1$, and furthermore, $\mathbb{E}[\|\langle X_t,g_j \rangle Z_t\|^2]\leq c_{\circ} \lambda_j^2$ and $\mathbb{E}[\|\langle Z_t,h_j \rangle X_t\|^2]\leq c_{\circ} \lambda_j^2$; \item $\langle g_j,\zeta \rangle \leq c_\circ j^{-\delta_{\zeta}}$.
\end{enumerate*}
\end{assumption}
The above assumptions are obvious adaptation of the conditions given by \cite{Hall2007} and \cite{seong2021functional}, which seem to be standard in the literature. Particularly, \cite{seong2021functional} established useful asymptotic results for the FFR model under Assumption \ref{assum2}, which are also useful in the considered FSR model. In fact, if Assumption \ref{assum2} is additionally satisfied, the consistency result given in Proposition \ref{prop1} can be established with $\alpha = o(T^{1/3})$ without requiring Assumption \ref{assum1}\ref{eq001a1}; this is a direct consequence of Theorem 3 of \cite{seong2021functional}, and in fact, adapting their result developed for the FFR model to the FSR  model is straightforward. In order to establish the local asymptotic normality result, we need more conditions, which are stated below:
\begin{assumption}\label{assum3}
\begin{enumerate*}[(i)]
\item $\alpha^{-1} = o(T^{1/3})$;  \item \label{assum3b} $\varsigma + \delta_{\zeta} > \rho/2+2$, $2\delta_{\zeta} \geq \rho+1$ and $T \alpha^{(2\varsigma+2\delta_{\zeta}-1)/\rho} = O(1)$; \item\label{assum3c} ${\theta}_{\KK}(\zeta)= \langle  {\zeta}, ({C}_{XZ}^\ast {C}_{XZ})^\dag{C}_{XZ}^\ast {C}_{ZZ} {C}_{XZ} ({C}_{XZ}^\ast {C}_{XZ})^\dag {\zeta} \rangle$.
\end{enumerate*}
\end{assumption} Particularly Assumption \ref{assum3}\ref{assum3b} requires $f$ and $\zeta$ to be smooth enough with respect to the eigenvectors $\{g_j\}_{j\geq 1}$ so that the entire map or element can be well approximated by those eigenvectors; this is a standard requirement in asymptotic analysis in the literature on functional linear models (see e.g., \citealp{seong2021functional} and reference therein). Assumption \ref{assum3}\ref{assum3c} requires a certain quantity depending on $\zeta$ to diverge to infinity, and this condition is expected to be satisfied for many possible choices of $\zeta$ (see the discussion given Remark 10 of \citealp{seong2021functional}).    We obtain the desired asymptotic normality result under this requirement. However, it turns out that even if such a smoothness condition is not satisfied, (i) \eqref{eqlocal} with $f(\zeta)$ beging replaced by $f\widehat{\Pi}_{\KK}(\zeta)$ holds as long as $\alpha$ decays at a sufficiently slow rate, and thus we can implement statistical inference on $f\widehat{\Pi}_{\KK}(\zeta)$ and (ii) $\widehat{\Pi}_{\KK}(\zeta)$ may be understood as the best linear approximation of $\zeta$ based on the covariation of $X_t$ and $Z_t$ (see Section 3.2 of \citealp{seong2021functional}).

The desired asymptotic normality result is given as follows:
\begin{proposition} \label{prop2} Under Assumptions \ref{assum1}-\ref{assum3}
\begin{equation}
\sqrt{\frac{T}{\hat{\sigma}^2_u\widehat{\theta}_{\KK}(\zeta)}}(\hat{f}(\zeta)-f(\zeta)) \to_d N(0,1),
\end{equation}
where $\hat{\sigma}^2_u=T^{-1}\sum_{t=1}^T (y_t-\hat{f}(X_t))$ and  $\widehat{\theta}_{\KK}(\zeta)= \langle  {\zeta}, (\widehat{C}_{XZ}^\ast \widehat{C}_{XZ})^\dag \widehat{C}_{XZ}^\ast \widehat{C}_{ZZ} \widehat{C}_{XZ} (\widehat{C}_{XZ}^\ast \widehat{C}_{XZ})^\dag {\zeta} \rangle$.
\end{proposition}
With some algebra, it can be shown that $\widehat{\theta}_{\KK}(\zeta)$, as given in Proposition \ref{prop2} can be written as 
\begin{equation} \label{eqtheta2}
\widehat{\theta}_{\KK}(\zeta) %= \langle \hat{\zeta}, \widehat{C}_{ZZ} \hat{\zeta} \rangle,  \quad \text{with} \quad  \hat{\zeta} = \sum_{j=1}^{\KK} \hat{\lambda}_j^{-2} \langle \hat{g}_j,\zeta \rangle \widehat{C}_{XZ}\hat{g}_j. 
=\frac{1}{T} \sum_{t=1}^T \left(\sum_{j=1}^{\KK} \hat{\lambda}_j^{-2} \langle \hat{g}_j, \zeta\rangle \langle \widehat{C}_{XZ}\hat{g}_j, Z_t\rangle\right)^2,
\end{equation}
which corresponds to \eqref{eqtheta} without demeaning the variables.

\subsubsection{Mathematical proofs}
\subsubsection*{Proof of Proposition \ref{prop1a}}
Using \eqref{eqreg2} and the expression given in \eqref{eqest1}, we find that 
	\begin{equation}
	\hat{f}  =   \widehat{C}_{Zy} \widehat{C}_{XZ} (\widehat{C}_{XZ}^\ast \widehat{C}_{XZ})^\dag	=  f \widehat{\Pi}_{\KK} +  \widehat{C}_{Zu} \widehat{C}_{XZ} (\widehat{C}_{XZ}^\ast \widehat{C}_{XZ})^\dag, \label{eq:b0}
	\end{equation}
	where $\widehat \Pi_{\KK}= \sum_{j=1} ^{\KK} \widehat g_j \otimes \widehat g_j$ as earlier introduced.  
	%Under our assumptions, we apply the central limit theorem for strongly mixing sequences (see, e.g., \citeauthor{heyde1974central}, \citeyear{heyde1974central}) and for martingale difference sequences to find that 
	%	$	T^{-1/2} \sum_{t=1}^T \left(\langle x_t,w_1 \rangle \langle z_t,w_2 \rangle - \langle  \mathcal C_{xz} w_1, w_2 \rangle  \right)  $ and $T^{-1/2}  \sum_{t=1}^T \langle z_t,w_1 \rangle \langle u_t,w_2 \rangle $ converge in distribution to a well defined random variable for all $w_1,w_2 \in \mathcal H$.
	%	\begin{align}\label{pfresult2}
		%		\frac{1}{\sqrt{T}} \sum_{t=1}^T \langle z_t,w_1 \rangle \langle u_t,w_2 \rangle
		%	\end{align}		
	%converges in distribution to a well defined random variable	for all $w_1$ and $w_2$. 
	%	Then, by applying Theorem 3 of \citet[Chapter 1]{skorohod2001}, it can be shown that 
	%	\begin{align}
		%		\sup_{T}	\frac{1}{\sqrt{T}} \sum_{t=1}^T (x_t \otimes  z_t - \mathcal C_{xz}) = O_p(1)\quad\text{and}\quad \quad \sup_{T}	\frac{1}{\sqrt{T}} \sum_{t=1}^T z_t \otimes  u_t = O_p(1); \label{eqcltref}
		%	\end{align}
	%	see also  Lemma A.1 of \cite{seo2020functional}. 
	As shown in the proof of Theorem 1 of \cite{seong2021functional}, we have  $\|\widehat{C}_{XZ} (\widehat{C}_{XZ}^\ast \widehat{C}_{XZ})^\dag\|_{\op} \leq \alpha^{-1/2}$ and $\|\widehat{\mathcal C}_{Zu}\|_{\HS}=O_p(T^{-1/2})$ by Assumption \ref{assum1}. We thus find that 
\begin{align}
	\|\widehat{f} - f\widehat{\Pi}_{\KK}\|_{\op} \leq \|\widehat{\mathcal C}_{Zu}\|_{\HS}  \|\widehat{C}_{XZ} (\widehat{C}_{XZ}^\ast \widehat{C}_{XZ})^\dag\|_{\op}  \leq O_p(\alpha^{-1/2} T^{-1/2}).
\end{align}
From the properties of the operator norm and that $\{\hat{g}_j\}_{j\geq 1}$ consists of an orthonormal basis, we find that 
\begin{equation}
\|f\widehat{\Pi}_{\KK} -f\|_{\op} \leq \sum_{j=1}^\infty \|f\widehat{\Pi}_{\KK}(\hat{g}_j) -f\hat({g}_j)\|. 
\end{equation}
Thus the proof becomes complete if $\sum_{j=1}^{\infty}\|f\widehat{\Pi}_{\KK}\hat{g}_j -f\hat{g}_j\| \to_p 0$ is shown. From  
	%	\begin{equation} \label{eqpf0006add2wadd0}
		%		\|\widehat{\mathcal A}- \mathcal A \widehat{\Pi}_{\K}\|_{\op} \leq O_p(\alpha^{-1/2} T^{-1/2}).
		%	\end{equation}
	%the following can be shown by 
	nearly identical arguments used to derive (8.63) of \cite{Bosq2000} and (S2.2) of \cite{seong2021functional}, we find that %and the property of the operator norm such that $\Vert \cdot \Vert_{\op} \leq \Vert \cdot \Vert_{\HS}$:
	\begin{equation}
	\sum_{j=1}^{\infty} \|f\widehat{\Pi}_{\KK}(\hat{g}_j) -f(\hat{g}_j)\|^2  \leq 	\sum_{j=\KK+1}^{\infty} \|f(\hat{g}_j)\|^2 \leq 	\sum_{j=\KK+1}^\infty \|f({g}_j)\|^2 + O_p(1)\|\widehat{ C}_{XZ}^\ast  \widehat{ C}_{XZ}- C_{XZ}^{\ast} C_{XZ}\|_{\op} \sum_{j=1}^{\KK} \tau_j.\label{eqpf0006add2wadd}
	\end{equation}
Since $\sum_{j=\KK+1}^\infty \|f(g_j)\|^2 < \infty$ under Assumption \ref{assum1}, $\sum_{j=\KK+1}^\infty \| f(g_j)|^2$ converges in probability to zero as $T$ gets larger (note that $\KK$ diverges as $T \to \infty$). In addition, 
$
		\|\widehat{ C}_{XZ}^\ast  \widehat{ C}_{XZ}- C_{XZ}^{\ast} C_{XZ}\|_{\op} \leq \|\widehat{ C}_{XZ}^\ast\|_{\op}\|\widehat{ C}_{XZ}- C_{XZ}\|_{\op} + \|\widehat{ C}_{XZ}^\ast- C_{XZ}^\ast\|_{\op}\| C_{XZ}\|_{\op} = O_p(T^{-1/2})$ as shown by (S2.3) of \cite{seong2021functional}. Combining all these results, we find that  \eqref{eqpf0006add2wadd} is $o_p(1)$ as desired.  \qed

\subsubsection*{Proof of Proposition \ref{prop2}}
Observe that $\widehat{\theta}_{\KK}$ in \eqref{eqtheta} can be equivalently written as follows:
\begin{equation}
\widehat{\theta}_{\KK}(\zeta)= \langle  {\zeta}, (\widehat{C}_{XZ}^\ast \widehat{C}_{XZ})^\dag\widehat{C}_{XZ}^\ast \widehat{C}_{ZZ} \widehat{C}_{XZ} (\widehat{C}_{XZ}^\ast \widehat{C}_{XZ})^\dag {\zeta} \rangle.
\end{equation}
We let ${\theta}_{\KK}(\zeta)= \langle  {\zeta}, ({C}_{XZ}^\ast {C}_{XZ})^\dag{C}_{XZ}^\ast {C}_{ZZ} {C}_{XZ} ({C}_{XZ}^\ast {C}_{XZ})^\dag {\zeta} \rangle$. From Theorem 4 (with its proof and Remark 10) of \cite{seong2021functional}, we find that Assumptions \ref{assum1}-\ref{assum3} lead us to the following:
\begin{equation} \label{eqconv1}
\sqrt{\frac{T}{\hat{\sigma}^2_u\widehat{\theta}_{\KK}(\zeta)}} (\hat{f}(\zeta)-f\widehat{\Pi}_{\KK}(\zeta)) \to_d N(0,1).
\end{equation}
Note that $\sqrt{T/\theta_{\KK}(\zeta)} (\hat{f}(\zeta)\widehat{\Pi}_{\KK}(\zeta)-f(\zeta))$ can be written as $\sqrt{T/\theta_{\KK}(\zeta)} (A_1+A_2+A_3+A_4)$, where $A_1 = \sum_{j=1}^{\KK} \langle \hat{g}_j-g_j^s,\zeta \rangle f(\hat{g}_j-g_j^s)$, $A_2 =\sum_{j=1}^{\KK} \langle g_j^s,\zeta \rangle f(\hat{g}_j-g_j^s)$,  $A_3 =\sum_{j=1}^{\KK} \langle \hat{g}_j-g_j^s,\zeta \rangle f(g_j)$, and $A_4 = f(\Pi_{\KK}-I) \zeta$, where $\Pi_{\KK} = \sum_{j=1}^{\KK} g_j \otimes g_j$ and $g_j^s = \sgn \langle g_j, \hat{g}_j \rangle g_j$. Under Assumptions \ref{assum1}-\ref{assum3}, it is shown by \cite{seong2021functional} (see (S2.11), (S2.16) and (S2.33)) that $\KK = O_p(\alpha^{-1/\rho})$ and 
\begin{align}
\|f(\hat{g}_j-g_j^s)\|^2 = O_p(T^{-1}) j^{\rho+2-2\varsigma},\\
\langle \hat{g}_j-g_j^s,\zeta \rangle^2 = O_p(T^{-1}) j^{-2\delta_{\zeta}+2 + \rho}.
\end{align} 
Combining these results with the conditions given in Assumption \ref{assum3}, it can be shown with nearly identical arguments used in \cite{seong2021functional} that $\|A_1\|, \|A_2\|$ and  $\|A_3\|$ are all $O_p(T^{-1/2})$ and, moreover, 
\begin{equation}
\|A_4\|^2\leq \sum_{j=\KK+1}^{\infty} \|\langle g_j,\zeta \rangle f(g_j) \|^2 %\leq\sum_{j=\KK+1}^{\infty} j^{-2\delta_{\zeta}} \|f(g_j) \| 
\leq  O(1)\sum_{j=\KK+1}^{\infty} j^{-2\delta_{\zeta}-2\varsigma} =  O((\KK+1)^{-2\delta_{\zeta}-2\varsigma+1})= O(\alpha^{(2\varsigma+2\delta_{\zeta}-1)/\rho}),
\end{equation}
where the first equality follows from the Euler-Maclaurin summation formula for the Riemann zera-function (see e.g., (5.6) of \citealp{ibukiyama2014euler}). 
Therefore, 
\begin{equation}\label{eqconv2}
\sqrt{T/\theta_{\KK}(\zeta)} (\hat{f}\widehat{\Pi}_{\KK}(\zeta)-f(\zeta)) = O_p(1/\sqrt{\theta_{\KK}(\zeta)}) + O(T^{-1/2}\alpha^{(\varsigma+\delta_{\zeta}-1/2)/\rho} /\sqrt{\theta_{\KK}(\zeta)}).
\end{equation}
Under Assumption \ref{assum3}, the above is $o_p(1)$. Lastly, we note that \cite{seong2021functional} shows that $|\widehat{\theta}_{\KK}(\zeta)- \theta_{\KK}(\zeta)| \to_p 0$ and replacing $ \theta_{\KK}(\zeta)$ with $\widehat{\theta}_{\KK}(\zeta)$ does not affect the results given in \eqref{eqconv1} and \eqref{eqconv2}. \qed

%From this result, we find that, if $f$ and $\zeta$ are smooth enough with respect to $\{g_j\}_{j\geq 1}$ (and thus $\varsigma$ and $\delta_{\zeta}$) are large enough, $\alpha$ is allowed to $\alpha = o(T^{1/3})$. 
